# Supplementary material for: M3GIA: A Cognition Inspired Multilingual and Multimodal General Intelligence Ability Benchmark
Source: arXiv:2406.05343 source file (2024-06-14)
Supplement: Supplementary file 1 [file multilingual_v2.tex]

\belowrulesep=0pt\aboverulesep=0pt

\begin{table}[ht]

  \centering
  \scriptsize
  \caption{\textbf{The GIA scores of different models accross the six languages.} The best in {\bf bold} and the second-best \underline{underlined}. The lower the better.}
  \label{tbl:multilingual}
  \setlength{\tabcolsep}{2.4mm}{
  \resizebox{1.0\linewidth}{!}{
        \begin{tabular}{>{\centering\arraybackslash}p{1.8cm}>{\centering\arraybackslash}p{0.032\linewidth}>{\centering\arraybackslash}p{0.032\linewidth}>
        {\centering\arraybackslash}p{0.032\linewidth}>{\centering\arraybackslash}p{0.032\linewidth}>{\centering\arraybackslash}p{0.032\linewidth}>{\centering\arraybackslash}p{0.032\linewidth}|>{\centering\arraybackslash}p{0.032\linewidth}>{\centering\arraybackslash}p{0.032\linewidth}>{\centering\arraybackslash}p{0.032\linewidth}>{\centering\arraybackslash}p{0.032\linewidth}>{\centering\arraybackslash}p{0.032\linewidth}>{\centering\arraybackslash}p{0.032\linewidth}>{\centering\arraybackslash}p{0.032\linewidth}}
        
        \customtop
        \multirow{2}{*}{Models}& \multicolumn{6}{c}{General Intelligence Abilitiy (GIA)}&\multicolumn{6}{c}{Normalized GIA Scores}\\
        \cmidrule{2-13}& En& Ch& Fr& Sp&Pt& Ko&En& Ch&  Fr&Sp& Pt& Ko\\
        
        \customhline
        Human& 16.01& 16.69& 19.52& 16.22&16.00& 18.05 
        &100.0& 100.0&  100.0&100.0& 100.0& 100.0\\
        
        \customhline
        \texttt{GPT-4o}& 13.85& 11.46& 12.37& 13.12&12.80& 13.01
        &86.5& 68.7&  63.3&80.9& 80.0& 72.1\\
        
        \texttt{GPT-4v}& 12.61& 10.95& 13.83& 14.04& 12.12& 12.25
        & 78.8& 65.6& 70.8& 86.5& 75.8&67.9\\
        
        \customhline
        \texttt{LLaVA-1.6-34b}& 11.47& 9.25& 11.35& 7.96&10.67& 9.04
        &71.6& 55.4&  58.1&49.1& 66.7& 50.1\\
        
        \texttt{LLaVA-1.6-13b}& 6.96& 6.89& 8.71& 7.75& 6.94& 7.75
        & 43.5& 41.3& 44.6& 47.8& 43.4&42.9\\
        
        \texttt{LLaVA-1.6-7b}& 6.75& 5.99& 7.67& 6.74&6.01& 5.93
        &42.1& 35.9&  39.3&41.5& 37.6& 32.9\\
        
        \customhline
        \texttt{Mini-Gemini-34b}& 11.00& 9.96& 12.75& 11.52&9.45& 10.69
        &68.7& 59.7&  65.3&71.0& 59.1& 59.2\\
        
        % \texttt{Mini-Gemini-7*8b}& 11.84& 8.96& 11.40& 10.76& 9.53& 9.88
        % & 73.9& 53.7& 58.4& 66.3& 59.6&54.8\\
        
        \texttt{Mini-Gemini-13b}& 8.68& 7.76& 8.65& 7.73& 7.10& 7.98
        & 54.2& 46.5& 44.3& 47.7& 44.4&44.2\\
        
        \texttt{Mini-Gemini-8b}& 9.32& 8.11& 11.25& 9.76& 8.99& 7.08
        & 58.2& 48.6& 57.6& 60.2& 56.2&39.3\\
        
        \customhline
        \texttt{Qwen-72b$^\dag$}& 11.68& 10.75& 10.20& 10.50& 9.71& 9.76
        & 72.9& 64.4& 52.2& 64.7& 60.7&54.1\\
        
        \texttt{Qwen-32b$^\dag$}& 10.58& 9.79& 9.62& 10.11& 9.25& 9.18
        & 66.1& 58.7& 49.3& 62.3& 57.8&50.9\\
        
        \texttt{Qwen-14b$^\dag$}& 8.46& 8.76& 9.15& 8.49& 8.79& 8.32
        & 52.8& 52.5& 46.9& 52.4& 54.9&46.1\\
        
        \texttt{Qwen-7b$^\dag$}& 8.56& 8.93& 8.98& 8.42& 8.77& 8.41
        & 53.4& 53.5& 46.0& 51.9& 54.8&46.6\\
        
        \texttt{Qwen-1.8b$^\dag$}& 7.34& 6.56& 8.01& 7.37& 6.49& 6.48
        & 45.8& 39.3& 41.0& 45.5& 40.6&35.9\\
        
        \custombot
        \end{tabular}}}
\end{table}
